# Supplementary material for: RLG-TPV: Radar- and LiDAR-Guided Tri-Perspective View Fusion for Camera-Radar 3D Object Detection
Source: arXiv:2608.29194 source file (2026-08-29)
Supplement: Supplementary file 1 [file X_suppl.tex]

\clearpage
\setcounter{page}{1}
\maketitlesupplementary
\appendix

% Letter-prefix supplementary floats.
\setcounter{table}{0}
\renewcommand{\thetable}{A\arabic{table}}
\setcounter{figure}{0}
\renewcommand{\thefigure}{A\arabic{figure}}


% ===============================================================
\section{Single-Plane BEV Controls}
\label{sec:suppl_bevsat}

Before introducing the TPV representation, we tested whether the observed single-plane performance could be improved by increasing BEV capacity or by applying height-aware auxiliary supervision after BEV projection. These experiments serve as controls for the placement of the geometric information used by RLG-TPV.

\textbf{Capacity control.}
Increasing the fused BEV width from 128 to 192 channels does not improve the CRN+VEMA configuration (\cref{tab:bev_sat}). Two independent runs reach 0.4842 and 0.4797 mAP, respectively, compared with 0.4886 for the 128-channel model; the run for which NDS is available also decreases from 0.5842 to 0.5775. We therefore found no evidence that simply widening the post-projection BEV resolves the performance limitation observed in this configuration.

\textbf{Fused-BEV supervision control.}
We additionally evaluated geometric class-occupancy targets as auxiliary losses directly on the fused BEV, i.e., after the vertical dimension had already been collapsed. Across 48 experimental configurations, results cluster around mAP $\approx0.484$. The strongest configuration, which also
includes a cross-modal LiDAR-camera distillation signal following the general setting of CRKD~\cite{crkd}, reaches 0.4889 mAP and 0.5880 NDS. Its mAP differs from the CRN+VEMA reference by only $+0.0003$, within the run-to-run variation observed in our experiments.

These controls do not establish a general limitation of BEV
representations. Rather, under the architecture studied here, neither additional BEV width nor height-aware supervision applied after projection provides a resolved improvement. This motivated applying geometric constraints earlier, while the corresponding spatial dimensions remain explicit in the representation.

\begin{table}[t]
\centering
\caption{Single-plane BEV controls. Increasing the fused-BEV width or
applying height-aware auxiliary supervision after BEV projection does not
produce a resolved mAP improvement over the CRN+VEMA reference.}
\label{tab:bev_sat}
\scriptsize
\setlength{\tabcolsep}{4pt}
\begin{tabular}{lcc}
\toprule
Configuration & mAP & NDS \\
\midrule
CRN baseline (released code)
& 0.4725 & 0.5617 \\

CRN + VEMA + vel.\ loss (128-ch)
& 0.4886 & 0.5842 \\

CRN + VEMA + vel.\ loss (192-ch, run A)
& 0.4842 & -- \\

CRN + VEMA + vel.\ loss (192-ch, run B)
& 0.4797 & 0.5775 \\

Fused-BEV height-occ.\ aux.\ (typical)
& $\approx0.484$ & -- \\

\quad + cross-modal distillation (best)
& 0.4889 & 0.5880 \\
\bottomrule
\end{tabular}
\end{table}


% ===============================================================
\section{Per-Class Results}
\label{sec:suppl_perclass}

\begin{table*}[t]
\centering
\caption{Per-class AP on the nuScenes validation set compared with the released CRN implementation used in our controlled experiments. \emph{CV}: construction vehicle; \emph{Ped}: pedestrian; \emph{Mot}: motorcycle; \emph{TC}: traffic cone.
$\Delta$ is the absolute AP difference in percentage points.}
\label{tab:perclass}
\scriptsize
\setlength{\tabcolsep}{3.5pt}
\begin{tabular}{lcccccccccc}
\toprule
& Car & Truck & Bus & Trailer & CV & Ped & Mot & Bicycle & TC & Barrier \\
\midrule
CRN baseline
& 71.9 & 42.7 & 53.3 & 23.9 & 15.8 & 46.2 & 54.1 & 45.9 & 57.7 & 61.0 \\

RLG-TPV (ours)
& 76.4 & 46.0 & 56.9 & 26.7 & 17.4 & 54.0 & 52.8 & 47.9 & 58.1 & 62.1 \\

$\Delta$
& $+4.5$ & $+3.3$ & $+3.6$ & $+2.8$ & $+1.6$
& $\mathbf{+7.8}$ & $-1.3$ & $+2.0$ & $+0.4$ & $+1.1$ \\
\bottomrule
\end{tabular}
\end{table*}

RLG-TPV improves nine of the ten classes relative to the released CRN baseline. The largest change occurs for pedestrian ($+7.8$ AP), while car, bus, and truck also show consistent gains. Motorcycle is the only class that decreases ($-1.3$ AP). The distribution of gains therefore does not indicate an improvement restricted to large or strongly radar-reflective
objects. Traffic-cone AP changes only slightly, which is also consistent with the limited $0.5$\,m vertical resolution of the side/front planes. We avoid attributing the class-level changes to individual modules because the final model combines the lifting, radar, and temporal modifications.


% ===============================================================
\section{Additional Ablations and Implementation Caveats}
\label{sec:suppl_disc}

\subsection{Height-Plane Supervision Target}

We compare two sources for the side/front supervision target while keeping the model configuration unchanged. The first rasterises the ground-truth 3D boxes, whereas the second rasterises class-labelled LiDAR occupancy, where each LiDAR return receives the class of the annotated box containing
it. Replacing the box-derived target with the LiDAR-derived target changes mAP by $+0.0005$ and NDS by $-0.0010$. Both changes are within the run-to-run variation observed in our experiments.

The result indicates that, for the present formulation, the sensor origin of the supervision target is not itself responsible for a measurable accuracy difference. This is useful practically: the corresponding side/front supervision can also be constructed from the training annotations when LiDAR is unavailable. We retain the LiDAR target in the reported model because it is a direct measurement of scene geometry, but
we do not claim an accuracy advantage over the box-derived target.


\subsection{Augmentation of Height-Plane Targets}

The height-plane targets are rasterized offline once for each training sample. The current data loader transforms these targets under horizontal flipping, but does not transform them under the rotation ($\pm22.5^\circ$) and scaling components of the BEV augmentation. A rotated training example can therefore pair rotated TPV features with an unrotated auxiliary target.

This mismatch affects only the auxiliary plane loss, whose weight is $0.5$; the detection targets and camera-depth supervision follow their corresponding augmentation correctly. Nevertheless, the mismatch introduces gradient noise whenever the horizontal location of the target is displaced relative to the predicted side/front plane. It is therefore a plausible
explanation for the weak isolated behavior of the plane-supervision term.

For this reason, the main paper treats the supervision experiments as evidence concerning the \emph{placement} and availability of the geometric constraint rather than claiming a resolved standalone accuracy gain from the LiDAR plane loss. A cleaner evaluation would generate the targets after augmentation or apply the identical transformation to the precomputed targets.


\subsection{3D Detection Head}

The TPV aggregation forms a height-resolved representation before reducing the vertical dimension for the CenterPoint detection head. We therefore tested whether retaining explicit height resolution for additional 3D-convolutional processing would improve detection.

Replacing the learned height collapse with a 3D-convolutional encoder decreases mAP by $0.0059$ and NDS by $0.0031$. The 3D encoder adds approximately 463\,K parameters, compared with approximately 2\,K parameters for the learned collapse. Truck, bus, and bicycle AP decrease, while mATE and mASE remain similar or improve slightly.

This negative result suggests that, in the architecture and task considered here, the benefit of the side/front planes does not require maintaining explicit height resolution throughout the detection head. The TPV representation can incorporate vertical information before being reduced to the BEV representation consumed by the standard detector.


% ===============================================================
\section{Model Size and Runtime}
\label{sec:suppl_eff}

\begin{table}[t]
\centering
\caption{Model size and reported runtime at ResNet-50 and
$256\times704$ input resolution. FPS values are measured on the hardware
reported by each source and therefore should not be interpreted as a
controlled latency comparison. Parameter counts for released models are
measured from their public implementations when not stated in the
corresponding paper.}
\label{tab:eff}
\scriptsize
\setlength{\tabcolsep}{3pt}
\begin{tabular}{lcccc}
\toprule
Method & Params & FPS & mAP & NDS \\
\midrule
CRN~\cite{crn}, paper
& -- & 20.4 & 0.490 & 0.560 \\

CRN, released code
& 61.4\,M & 22.7 & 0.473 & 0.562 \\

RLG-TPV (ours)
& 67.5\,M & 15.7 & 0.498 & 0.596 \\
\bottomrule
\end{tabular}
\end{table}

\cref{tab:eff} is included for model-scale transparency rather than as a controlled efficiency comparison. The reported frame rates originate from different hardware and implementations: CRN reports 20.4\,FPS, its released configuration measures 22.7\,FPS, and our model measures 15.7\,FPS on an RTX 4090. A common-hardware benchmark would be required for a direct latency comparison.

RLG-TPV contains 67.5\,M parameters compared with 61.4\,M for
the released CRN model. Approximately 0.8\,M parameters in our instantiated model belong to baseline radar-view-transform components that are not used by the final architecture; pruning unused modules would reduce the deployed parameter count accordingly.  Training the final RLG-TPV model takes approximately 87 GPU-hours on one RTX 4090 for the reported
24-epoch schedule.


% ===============================================================
\section{VEMA Baseline Control}
\label{sec:vema}

\begin{table}[t]
\centering
\caption{Effect of VEMA on the single-plane CRN baseline used to initialise
the early TPV experiments.}
\label{tab:vema}
\scriptsize
\begin{tabular}{lcc}
\toprule
Configuration & mAP & NDS \\
\midrule
CRN (released code)
& 0.4725 & 0.5617 \\

\textbf{CRN + VEMA}
& \textbf{0.4886} & \textbf{0.5842} \\
\midrule
$\Delta$
& $+0.0161$ & $+0.0225$ \\
\bottomrule
\end{tabular}
\end{table}

VEMA injects radar Doppler information into the positional encoding of the fused BEV and substantially improves the single-plane CRN configuration (\cref{tab:vema}). We therefore use CRN+VEMA as the strongest available single-plane warm start for development of the attentive lift.

VEMA is subsequently omitted when constructing the final multi-plane architecture, where motion information is already incorporated through multi-frame features and DGTF directly uses measured radar Doppler during temporal alignment. Importantly, the transition in \cref{tab:tpv} also introduces other architectural changes, so it does not constitute an
isolated VEMA ablation in the TPV model. We therefore use
\cref{tab:vema} only to document the role of VEMA in the single-plane baseline and do not claim a separately measured gain or loss from its removal in RLG-TPV.

% ===============================================================
\section{Additional Qualitative Results}
\label{sec:suppl_qual}

\begin{figure*}[t]
\centering
\includegraphics[width=\textwidth]{figures/fig_qual_rain.png}\\[0.45em]
\includegraphics[width=\textwidth]{figures/fig_qual_rain_street.png}
\caption{Qualitative comparison in rain. Columns are ground truth (left), the
  released CRN~\cite{crn} implementation (middle), and RLG-TPV (right);
  ground-truth boxes are green and predictions blue in both model columns, which
  are therefore distinguished by column rather than by colour, unlike
  \cref{fig:qual}. Map and LiDAR points are shown for visualisation only.
  \textbf{Top:} a wet
  intersection with reflections on the road surface. \textbf{Bottom:} a dense
  urban street with vehicles parked along both sides. The main-paper scenes are
  shown in \cref{fig:qual}.}
\label{fig:qual_suppl}
\end{figure*}

\cref{fig:qual_suppl} shows two rain scenes, a condition in which image evidence is degraded by reflections and reduced contrast while radar measurements remain available. Both models detect the parked vehicles along the street in the second scene, and the visible differences again concern the orientation consistency of neighboring boxes and isolated predictions in regions with few
returns. These examples are provided for completeness; we do not draw quantitative conclusions from them, since the evaluation protocol of the main paper is not stratified by weather condition.
